# Supplementary material for: Query-driven Relevant Paragraph Extraction from Legal Judgments
Source: arXiv:2404.00595 source file (2024-03-31)
Supplement: Supplementary file 1 [file appendix.tex]

\section{Appendix}
